# Supplementary material for: A Secure Blockchain-Assisted Framework for Real-Time Maritime Environmental Compliance Monitoring
Source: arXiv:2503.08707 source file (2025-03-10)
Supplement: Supplementary file 1 [file supplement.tex]

Furthermore, Figure \ref{fig:dca&l-a} gives the validation and training accuracy of the model based on the number of epochs, and Figure \ref{fig:dca&l-b} provides the validation and training loss of the model based on the number of epochs.
\begin{figure*}
    \centering
    \begin{subfigure}[b]{0.48\textwidth}
    \includegraphics[height=6.4cm, width=8.5cm]{figures/accuracycifar10deepconfuse.eps}
    \caption{Training and validation accuracy of our model trained with poisoned CIFAR-10 data with Deepconfuse.}
    \label{fig:dca&l-a}
    \end{subfigure}
    \begin{subfigure}[b]{0.48\textwidth}
    \includegraphics[height=6.4cm, width=8.5cm]{figures/losscifar10deepconfuse.eps}
    \caption{Training and validation loss of our model trained with poisoned CIFAR-10 data with Deepconfuse.}
    \label{fig:dca&l-b}
    \end{subfigure}
    \caption{The accuracy and loss curves show that our model is overfitting. The training accuracy and loss is a smooth curve. However, the validation accuracy and loss are not.}
    \label{fig:dca&l}
\end{figure*}
